# Supplementary material for: Pentagon Wilson loop with Lagrangian insertion at two loops in ${\mathcal N}=4$ super Yang-Mills theory
Source: arXiv:2204.00329 ancillary file (2022-04-01)
Supplement: Supplementary file 1 [file tables.pdf]

# The observed sign patterns of the two-loop functions in the numerical experiments in the Euclidean region with $\epsilon_5 > 0$

The signs of the leading singularities  $(-|++-++)$  and  $(-|-++++-)$ , corresponding to Tab. 1 and 2, respectively, are invariant under reflection  $\rho$ . The sign patterns of the two-loop function in Tab. 1 and 2 are also closed under reflection  $\rho$ .

| $g_0^{(2)}$ | $g_1^{(2)}$ | $g_2^{(2)}$ | $g_3^{(2)}$ | $g_4^{(2)}$ | $g_5^{(2)}$ |
|-------------|-------------|-------------|-------------|-------------|-------------|
| +           | -           | -           | +           | -           | -           |
| +           | -           | +           | +           | -           | +           |
| +           | +           | -           | +           | +           | -           |
| +           | -           | -           | +           | +           | -           |
| +           | -           | +           | +           | -           | -           |
| +           | +           | -           | +           | +           | +           |
| +           | +           | +           | +           | -           | +           |
| -           | +           | +           | +           | +           | +           |
| -           | +           | -           | +           | -           | +           |
| -           | -           | -           | +           | -           | -           |
| -           | +           | +           | +           | -           | +           |
| -           | +           | -           | +           | +           | +           |
| -           | +           | +           | +           | -           | -           |
| -           | -           | -           | +           | +           | +           |
| -           | -           | +           | +           | -           | +           |
| -           | +           | -           | +           | +           | -           |
| -           | -           | +           | +           | -           | -           |
| -           | -           | -           | +           | +           | -           |
| -           | +           | -           | +           | -           | -           |
| -           | -           | -           | +           | -           | +           |

Table 1: Observed 20 sign patterns of the two-loop pure functions in the subregion (B) with  $\epsilon_5 > 0$ , i.e. the leading singularities  $(r_{5,0}|r_{5,1}, r_{5,2}, r_{5,3}, r_{5,4}, r_{5,5})$  take signs  $(-|++-++)$ .

| $g_0^{(2)}$ | $g_1^{(2)}$ | $g_2^{(2)}$ | $g_3^{(2)}$ | $g_4^{(2)}$ | $g_5^{(2)}$ |
|-------------|-------------|-------------|-------------|-------------|-------------|
| +           | +           | +           | +           | +           | +           |
| +           | +           | +           | -           | +           | +           |
| +           | +           | -           | +           | -           | +           |
| +           | +           | -           | -           | -           | +           |
| +           | -           | +           | +           | +           | -           |
| +           | +           | +           | -           | -           | +           |
| +           | +           | -           | -           | +           | +           |
| +           | -           | +           | +           | +           | +           |
| +           | +           | +           | +           | +           | -           |
| +           | -           | -           | -           | -           | +           |
| +           | +           | -           | -           | -           | -           |
| -           | +           | +           | +           | +           | +           |
| -           | +           | +           | -           | +           | +           |
| -           | +           | -           | +           | -           | +           |
| -           | +           | -           | -           | -           | +           |
| -           | +           | +           | +           | -           | +           |
| -           | +           | -           | +           | +           | +           |
| -           | +           | +           | -           | -           | +           |
| -           | +           | -           | -           | +           | +           |
| -           | -           | +           | +           | +           | +           |
| -           | +           | +           | +           | +           | -           |
| -           | -           | -           | -           | -           | +           |
| -           | +           | -           | -           | -           | -           |

Table 2: Observed 23 sign patterns of the two-loop pure functions in the subregion (C) with  $\epsilon_5 > 0$ , i.e. the leading singularities  $(r_{5,0}|r_{5,1}, r_{5,2}, r_{5,3}, r_{5,4}, r_{5,5})$  take signs  $(-|-+++-)$ .
